# Supplementary material for: New symplectic singularities from $SU(2)$ gauge theories
Source: arXiv:2608.06451 source file (2026-08-06)
Supplement: Supplementary file 2 [file Appendix_C.tex]

\section{Normalisers of Closed Subgroups of \texorpdfstring{$\mathrm{SU}(2)$}{\surm(2)}}
\todo[inline]{consider removing}
We classify the normaliser of each closed subgroup \(G\leq \mathrm{SU}(2)\), up to conjugacy. 
The word ``closed'' is important: without this assumption there are also dense subgroups, 
and no finite classification table is available.

Let
\begin{equation}
T=
\left\{
\begin{pmatrix}
z & 0\\
0 & z^{-1}
\end{pmatrix}
:\ |z|=1
\right\}
\cong \mathrm{U}(1)
\end{equation}
be the standard maximal torus of \(\mathrm{SU}(2)\). Its normaliser is
\begin{equation}
N(T)=N_{\mathrm{SU}(2)}(T)
=\{g\in \mathrm{SU}(2):gTg^{-1}=T\}.
\end{equation}
Explicitly,
\begin{equation}
N(T)=T\cup wT,
\qquad
w=
\begin{pmatrix}
0 & -1\\
1 & 0
\end{pmatrix}.
\end{equation}
The element \(w\) acts on \(T\) by inversion:
\begin{equation}
w
\begin{pmatrix}
z & 0\\
0 & z^{-1}
\end{pmatrix}
w^{-1}
=
\begin{pmatrix}
z^{-1} & 0\\
0 & z
\end{pmatrix}.
\end{equation}
Hence
\begin{equation}
N(T)/T\cong \mathbb{Z}_2,
\end{equation}
which is the Weyl group of \(\mathrm{SU}(2)\).

The finite closed subgroups of \(\mathrm{SU}(2)\) are the cyclic groups \(\mathbb{Z}_n\), 
the binary dihedral groups \(\mathrm{Dic}_n\), and the binary tetrahedral, octahedral, 
and icosahedral groups \(2\mathrm{T}\), \(2\mathrm{O}\), and \(2\mathrm{I}\). Together 
with \(T\), \(N(T)\), and \(\mathrm{SU}(2)\), these give all closed subgroups of 
\(\mathrm{SU}(2)\), up to conjugacy.

\begin{table}[h]
\centering
\renewcommand{\arraystretch}{1.35}
\begin{tabular}{c|c|c|c}
\hline
\(G\leq \mathrm{SU}(2)\)
& Conditions / convention
& \(N_{\mathrm{SU}(2)}(G)\)
& \(N_{\mathrm{SU}(2)}(G)/G\)
\\
\hline
\(\{1\}=\mathbb{Z}_1\)
& Trivial subgroup
& \(\mathrm{SU}(2)\)
& \(\mathrm{SU}(2)\)
\\
\hline
\(\mathbb{Z}_2=\{\pm I\}\)
& Centre of \(\mathrm{SU}(2)\)
& \(\mathrm{SU}(2)\)
& \(\mathrm{SO}(3)\)
\\
\hline
\(\mathbb{Z}_n\leq T\)
& \(n\geq 3\)
& \(N(T)\)
& \(N(T)/\mathbb{Z}_n\)
\\
\hline
\(\mathrm{Dic}_2=\mathrm{Q}_8\)
& Binary dihedral of order \(8\)
& \(2\mathrm{O}\)
& \(\mathrm{S}_3\)
\\
\hline
\(\mathrm{Dic}_n\)
& \(n\geq 3,\ |\mathrm{Dic}_n|=4n\)
& \(\mathrm{Dic}_{2n}\)
& \(\mathbb{Z}_2\)
\\
\hline
\(2\mathrm{T}\)
& Binary tetrahedral, order \(24\)
& \(2\mathrm{O}\)
& \(\mathbb{Z}_2\)
\\
\hline
\(2\mathrm{O}\)
& Binary octahedral, order \(48\)
& \(2\mathrm{O}\)
& \(1\)
\\
\hline
\(2\mathrm{I}\)
& Binary icosahedral, order \(120\)
& \(2\mathrm{I}\)
& \(1\)
\\
\hline
\(T\cong \mathrm{U}(1)\)
& Maximal torus
& \(N(T)\)
& \(\mathbb{Z}_2\)
\\
\hline
\(N(T)\)
& Normaliser of the maximal torus
& \(N(T)\)
& \(1\)
\\
\hline
\(\mathrm{SU}(2)\)
& Whole group
& \(\mathrm{SU}(2)\)
& \(1\)
\\
\hline
\end{tabular}
\caption{Normalisers of closed subgroups of \(\mathrm{SU}(2)\), up to conjugacy.}
\end{table}

The first two cyclic cases are exceptional. The trivial subgroup and the centre 
\(\{\pm I\}\) are normal in all of \(\mathrm{SU}(2)\), so their normalisers are the whole group:
\begin{equation}
N_{\mathrm{SU}(2)}(\{1\})=\mathrm{SU}(2),
\qquad
N_{\mathrm{SU}(2)}(\{\pm I\})=\mathrm{SU}(2).
\end{equation}
Therefore
\begin{equation}
N_{\mathrm{SU}(2)}(\{1\})/\{1\}\cong \mathrm{SU}(2),
\qquad
N_{\mathrm{SU}(2)}(\{\pm I\})/\{\pm I\}\cong \mathrm{SO}(3).
\end{equation}

For \(n\geq 3\), a cyclic subgroup \(\mathbb{Z}_n\leq T\) determines the torus 
\(T\) uniquely. Thus any element normalising \(\mathbb{Z}_n\) must normalise 
\(T\), and hence
\begin{equation}
N_{\mathrm{SU}(2)}(\mathbb{Z}_n)=N(T).
\end{equation}
The quotient is therefore
\begin{equation}
N_{\mathrm{SU}(2)}(\mathbb{Z}_n)/\mathbb{Z}_n=N(T)/\mathbb{Z}_n.
\end{equation}
Equivalently, this quotient fits into the exact sequence
\begin{equation}
1\longrightarrow T/\mathbb{Z}_n
\longrightarrow N(T)/\mathbb{Z}_n
\longrightarrow \mathbb{Z}_2
\longrightarrow 1.
\end{equation}
Since \(T/\mathbb{Z}_n\cong \mathrm{U}(1)\), this is a one-dimensional compact group with two connected 
components. More explicitly,
\begin{equation}
N(T)/\mathbb{Z}_n\cong
\begin{cases}
\mathrm{O}(2), & n \text{ even},\\
N(T)\cong \mathrm{Pin}(2), & n \text{ odd}.
\end{cases}
\end{equation}

The binary dihedral groups require a small convention. We write \(\mathrm{Dic}_n\) for 
the binary dihedral group of order \(4n\). The group \(\mathrm{Dic}_2\) is the quaternion 
group:
\begin{equation}
\mathrm{Dic}_2=\mathrm{Q}_8.
\end{equation}
Its normaliser is larger than the generic binary dihedral case:
\begin{equation}
N_{\mathrm{SU}(2)}(\mathrm{Q}_8)=2\mathrm{O},
\end{equation}
and the quotient is
\begin{equation}
2\mathrm{O}/\mathrm{Q}_8\cong \mathrm{S}_3.
\end{equation}
For \(n\geq 3\), one has
\begin{equation}
N_{\mathrm{SU}(2)}(\mathrm{Dic}_n)=\mathrm{Dic}_{2n},
\end{equation}
so that
\begin{equation}
N_{\mathrm{SU}(2)}(\mathrm{Dic}_n)/\mathrm{Dic}_n\cong \mathbb{Z}_2.
\end{equation}

For the binary polyhedral groups, the tetrahedral group \(2\mathrm{T}\) is normal inside the 
binary octahedral group \(2\mathrm{O}\), and this gives
\begin{equation}
N_{\mathrm{SU}(2)}(2\mathrm{T})=2\mathrm{O},
\qquad
N_{\mathrm{SU}(2)}(2\mathrm{T})/(2\mathrm{T})\cong \mathbb{Z}_2.
\end{equation}
The binary octahedral and binary icosahedral groups are self-normalising:
\begin{equation}
N_{\mathrm{SU}(2)}(2\mathrm{O})=2\mathrm{O},
\qquad
N_{\mathrm{SU}(2)}(2\mathrm{I})=2\mathrm{I}.
\end{equation}
Thus
\begin{equation}
N_{\mathrm{SU}(2)}(2\mathrm{O})/(2\mathrm{O})\cong 1,
\qquad
N_{\mathrm{SU}(2)}(2\mathrm{I})/(2\mathrm{I})\cong 1.
\end{equation}

Finally, for the infinite closed subgroups, the maximal torus has normaliser 
\(N(T)\), so
\begin{equation}
N_{\mathrm{SU}(2)}(T)/T\cong \mathbb{Z}_2.
\end{equation}
The groups \(N(T)\) and \(\mathrm{SU}(2)\) are self-normalising:
\begin{equation}
N_{\mathrm{SU}(2)}(N(T))=N(T),
\qquad
N_{\mathrm{SU}(2)}(\mathrm{SU}(2))=\mathrm{SU}(2).
\end{equation}
Therefore
\begin{equation}
N_{\mathrm{SU}(2)}(N(T))/N(T)\cong 1,
\qquad
N_{\mathrm{SU}(2)}(\mathrm{SU}(2))/\mathrm{SU}(2)\cong 1.
\end{equation}
